# Supplementary material for: Structured Prediction Cascades
Source: arXiv:1208.3279 source file (2012-08-06)
Supplement: Supplementary file 1 [file appendix.tex]

\appendix
\newcommand{\tphi}{\tilde{\phi}}

\section{Video Clips}

Included in the supplemental archive is a sample of test results {\tt
  testset\_samples.mp4}:
\begin{itemize}
\item The cyan lines indicate the best of the top
$K=4$ hypotheses for the ensemble; the red lines indicate the best of
top $K=4$ hypotheses for the single frame SC model.
\item The point clouds show the top 150 unfiltered locations for each
  limb according to the ensemble model.
\item The video illustrates the significant {\em qualitative} increase
  in accuracy of the ensemble over single-frame methods, eliminating
  the ``jitter'' due to the lack of smoothing.
\end{itemize}

\section{Proof of Theorem 1}

We prove the theorem by applying the following result from \cite{bartlettM02}:
\begin{thm}[Bartlett and Mendelson, 2002]
  \label{thm:genbound}
  Consider a loss function $\mathcal{L}$ and a dominating cost
  function $\phi$ such that $\cL(y,x) \le \phi(y,x)$. Let $F:
  \mathcal{X} \mapsto \mathcal{A}$ be a class of functions. Then for
  any integer $n$ and any $0 < \delta < 1$, with probability $1 -
  \delta$ over samples of length $n$, every $f$ in $F$ satisfies
  \begin{equation}
    \label{eq:genbound}
      \bbE\cL(Y,f(X)) \le  \hat{\bbE}_n \phi(Y,f(X)) + R_n(\tilde{\phi} \;\circ\; F) + \sqrt{ \frac{8 \ln(2/\delta)}{n} },
  \end{equation}
  where $\tilde{\phi} \circ F$ is a centered composition of $\phi$
  with $f \in F$, $\tilde{\phi} \circ f = \phi(y,f(X)) - \phi(y,0)$.

  Furthermore, there are absolute constants $c$ and $C$ such that for
  every class $F$ and every integer $n$,
  \begin{equation}
    \label{eq:rad_to_gaus}
    cR_n(F) \le G_n(F) \le C \ln  n R_n(F).
  \end{equation}
  Let $\cA = \reals^m$ and $F: \cX \to \cA$ be a class of functions
  that is the direct sum of real-valued classes $F_1, \dots,
  F_m$. Then, for every integer $n$ and every sample $(X_1,Y_1), \dots,
  (X_n,Y_n)$,
  \begin{equation}
    \label{eq:multi_gaus}
    \hG_n(\tphi \circ F) \le 2L \sum_{i=1}^m \hG_n(F_i).
  \end{equation}
  Let $F = \{x \mapsto \bw^\top\bft(x,\cdot) \mid ||\bw||_2 \le B,
  ||\bft(x,\cdot)||_2 \le 1\}$. Then,
  \begin{equation}
    \label{eq:lingaus}
    \hat{G}_n(F) \le \frac{2B}{\sqrt{n}}.
  \end{equation}
\end{thm}
Proving the theorem reduces to analyzing the Lipschitz constant of the
dominating cost function,
$$\phi(y,\ssp) = r_\gamma\left(\frac{1}{P}\sum_p \pscore{y} -\pthr{x}\right).$$
Let $\phi_p(y,\theta_p) = \pscore{y} - \pthr{x}$. If we let $\ssp^p$ be a
$m$-dimensional vector whose elements correspond to the scores of
every possible clique assignment given $\theta_p$, then we can rewrite
$\phi_p$ as the following:
$$\phi_p(y,\ssp^p) = \ang{y,\ssp^p} - \thr,$$
where we consider $y$ to be a binary $m$-dimensional vector that
selects the active clique assignments in the output $y$. We now make
use of the following lemma from \cite{weiss10}:
\begin{lem}[Weiss \& Taskar, 2010]
  \label{lem:useful}
  Let $\ssp$ be a vector of clique assignment scores. Let $g(\ssp) =
  \ang{y,\ssp} - \thr.$ Then $g(u) - g(v) \le \sqrt{2\ell}||u-v||_2$.
\end{lem}
\begin{lem}
  \label{lem:combined}
  $\phi(y,\cdot)$ is Lipschitz with constant $\sqrt{2\ell}$.
\end{lem}
\begin{proof}
  By Lemma \ref{lem:useful}, we see that $\phi_p$ is Lipschitz with
  constant $\sqrt{2\ell}$. Since $\phi$ is simply the average of $P$
  such functions, the Lipschitz of $\phi$ must be $\sqrt{2\ell}$ as
  well.
\end{proof}
Finally, to prove the theorem, we note that the loss function
$\cL(\theta, \ang{X,Y}, \alpha)$ can be represented as a function in
$\reals^{mP}$ space by contatenating the clique scoring vectors of
each of the $P$ individual sub-models. Substituing $mP$ for the
dimensionality of the loss function ($m$ in Theorem
\ref{thm:genbound}) yields the desired result.

%%% Local Variables: 
%%% mode: latex
%%% TeX-master: "../supplemental"
%%% End: 
